# Supplementary material for: Can Cascades be Predicted?
Source: arXiv:1403.4608 source file (2014-03-18)
Supplement: Supplementary file 1 [file 070appendix.tex]

% !TEX root = paper-fb.tex

\subsection{Variable importance}

\begin{figure}[h]
\centering
\includegraphics[width=\linewidth]{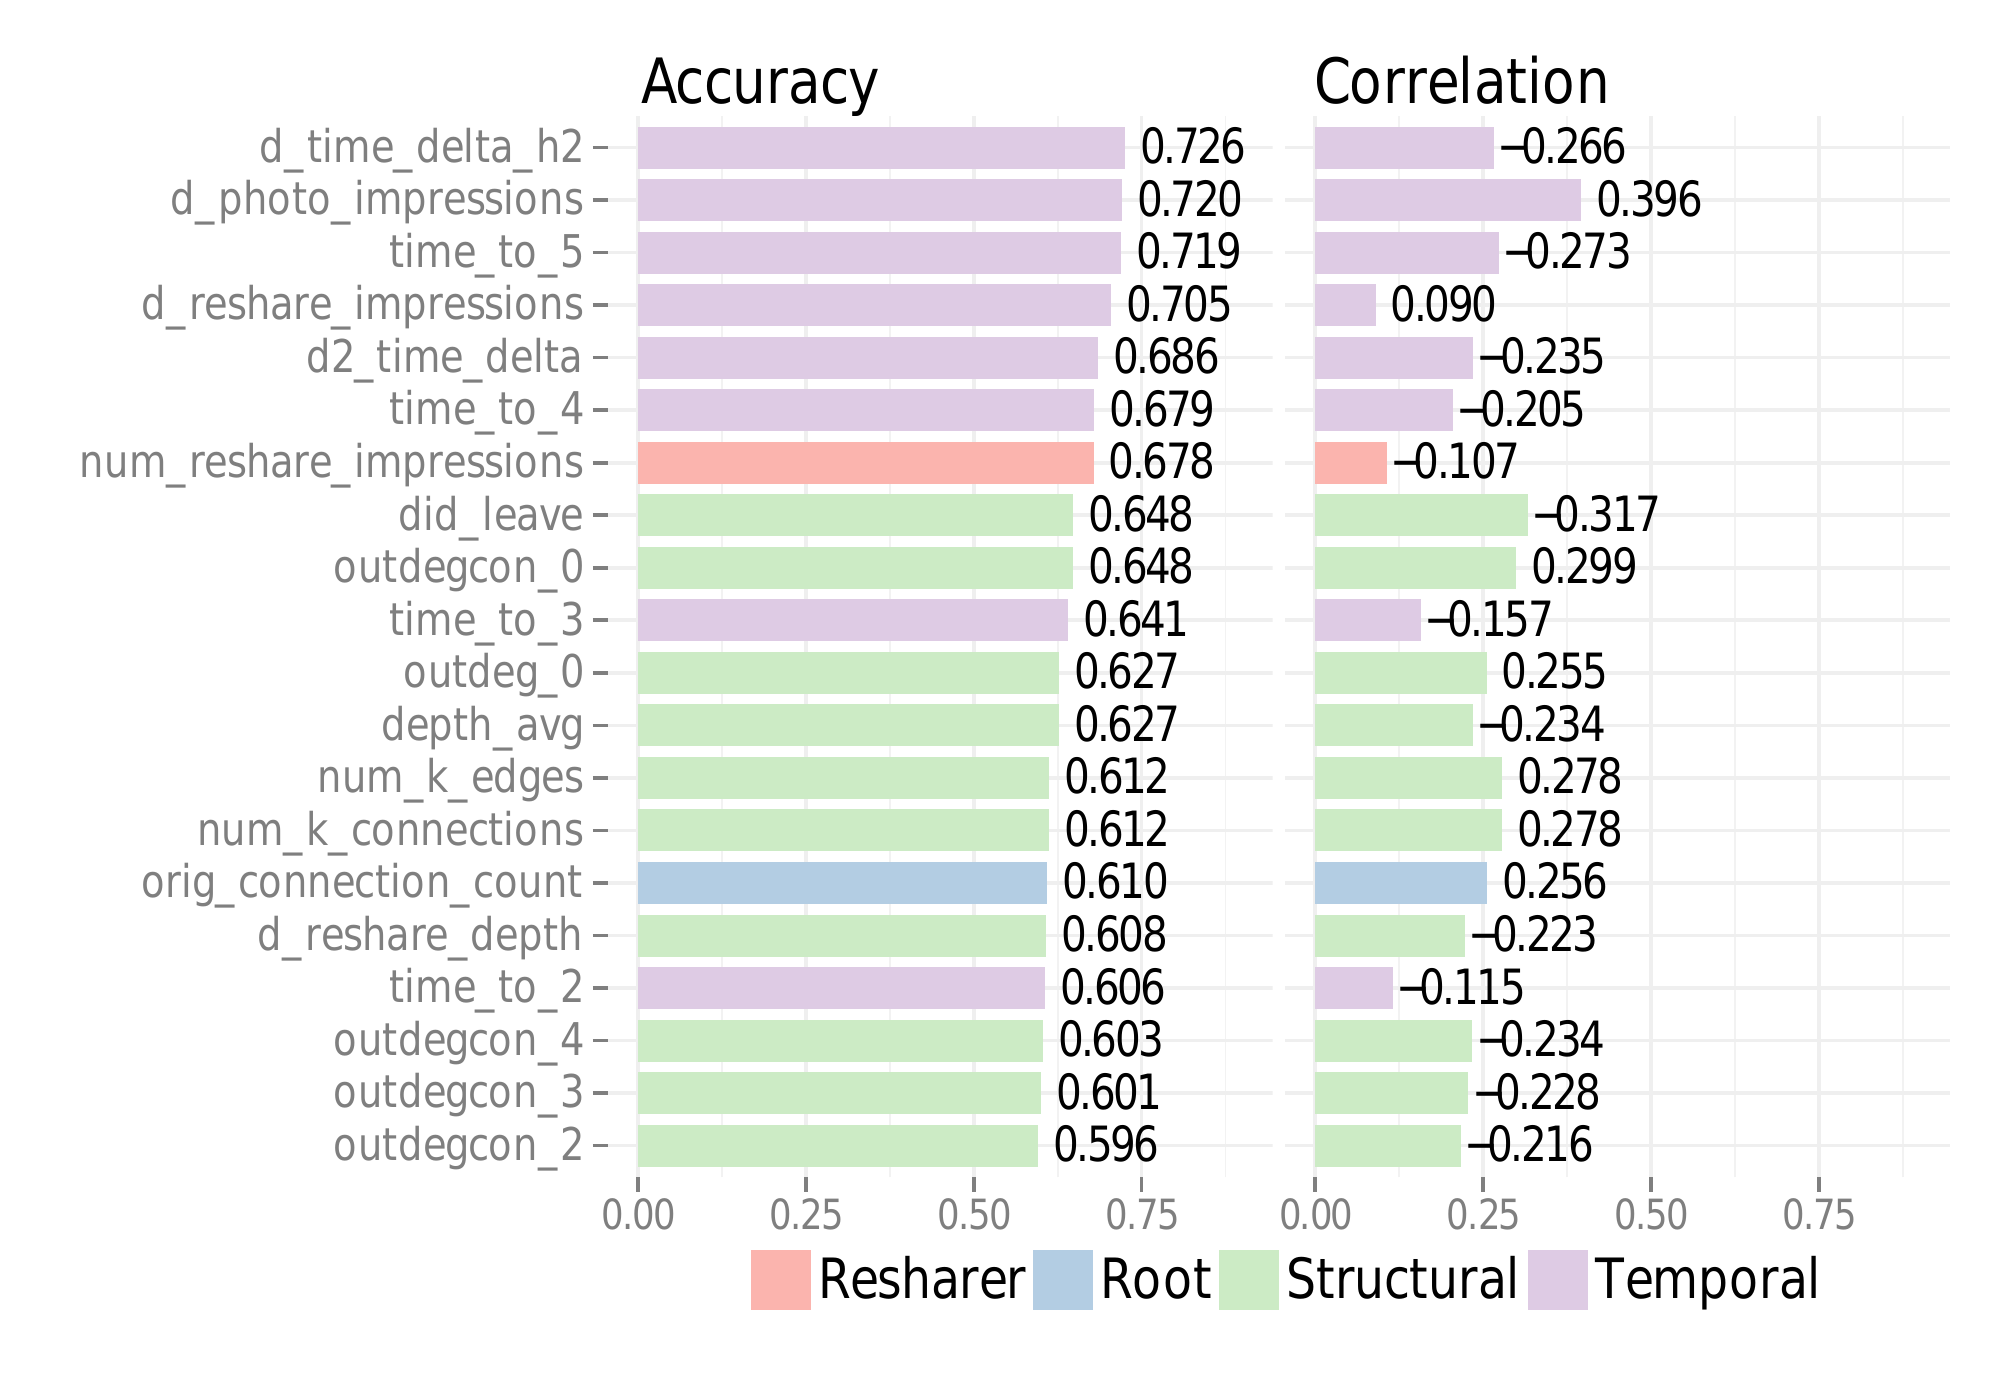}
\caption{The 20 most accurate individual predictors of cascade size. Individually, temporal and structural features, as well as those that relate to the number of impressions photos or reshares receive, are the most accurate predictors of cascade size.}
\label{fig:paper_indiv_predcor}
\end{figure}

When using features individually to predict whether a cascade will double in size, we find that temporal features are most indicative of future growth (Figure \ref{fig:paper_indiv_predcor}).
Nevertheless, structural features also perform comparably, and also are significantly correlated with the log-transformed cascade size.

\begin{figure}[h]
\centering
\includegraphics[width=\linewidth]{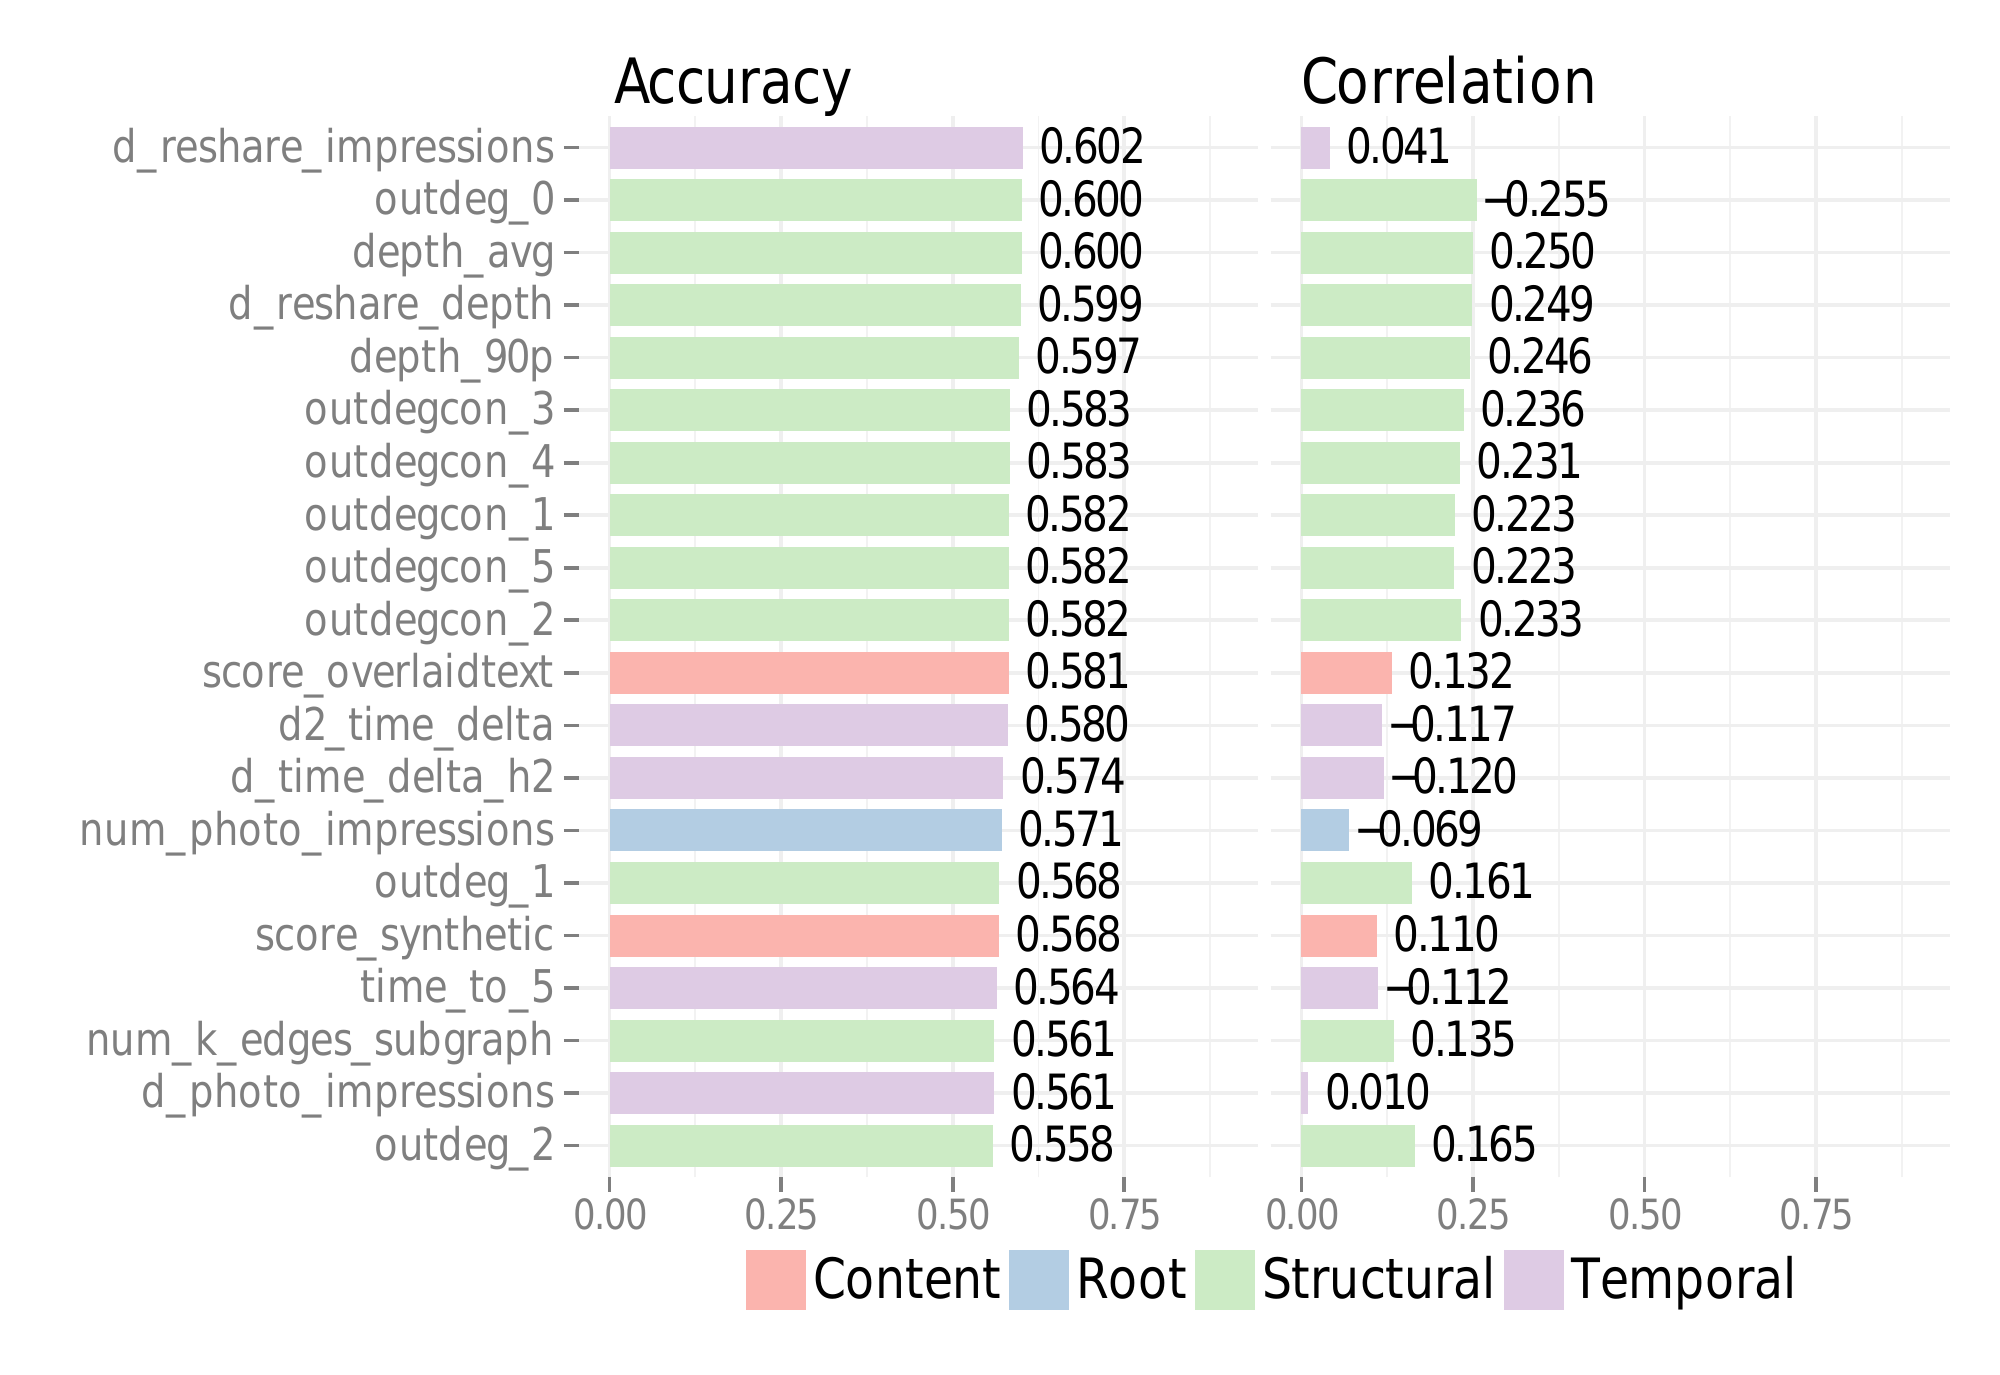}
\caption{The 20 most accurate individual predictors of the Wiener index.}
\label{fig:paper_indiv_predcor_avgdist}
\end{figure}

\subsection{Content type dataset properties}

\begin{figure}[h]
\centering
\includegraphics[width=\linewidth]{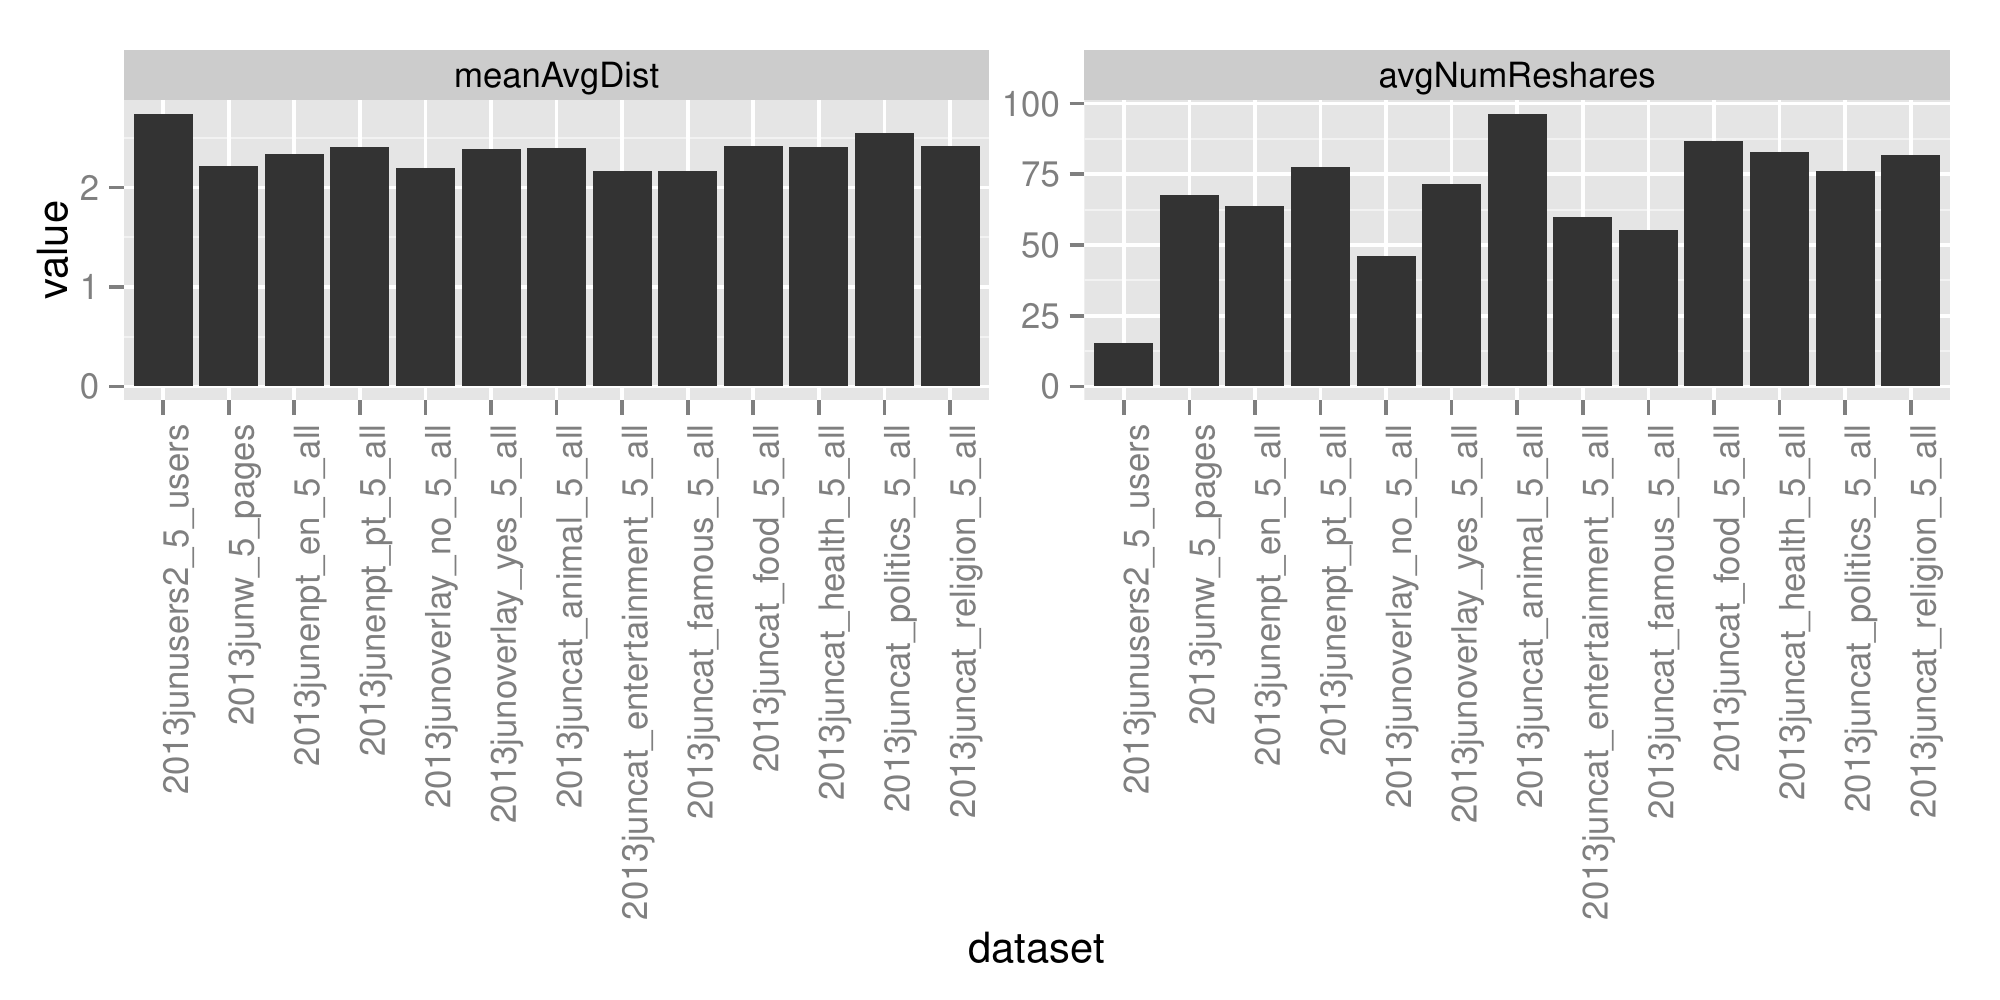}
\caption{\todo{Mean Avg Distance and Mean Num Reshares for Different Datasets}}
\label{fig:datasetstats}
\end{figure}

Some summary statistics are in Figure \ref{fig:datasetstats}. For creating a dataset with different categories, we matched photos to specific Wikipedia articles, and in turn matched these to categories, using Wikipedia category data. We divided these matched reshares into seven categories: animal, entertainment, famous people (excluding religious and political figures), food, health, politics and religion.

\begin{figure}
\centering
\includegraphics[width=\linewidth]{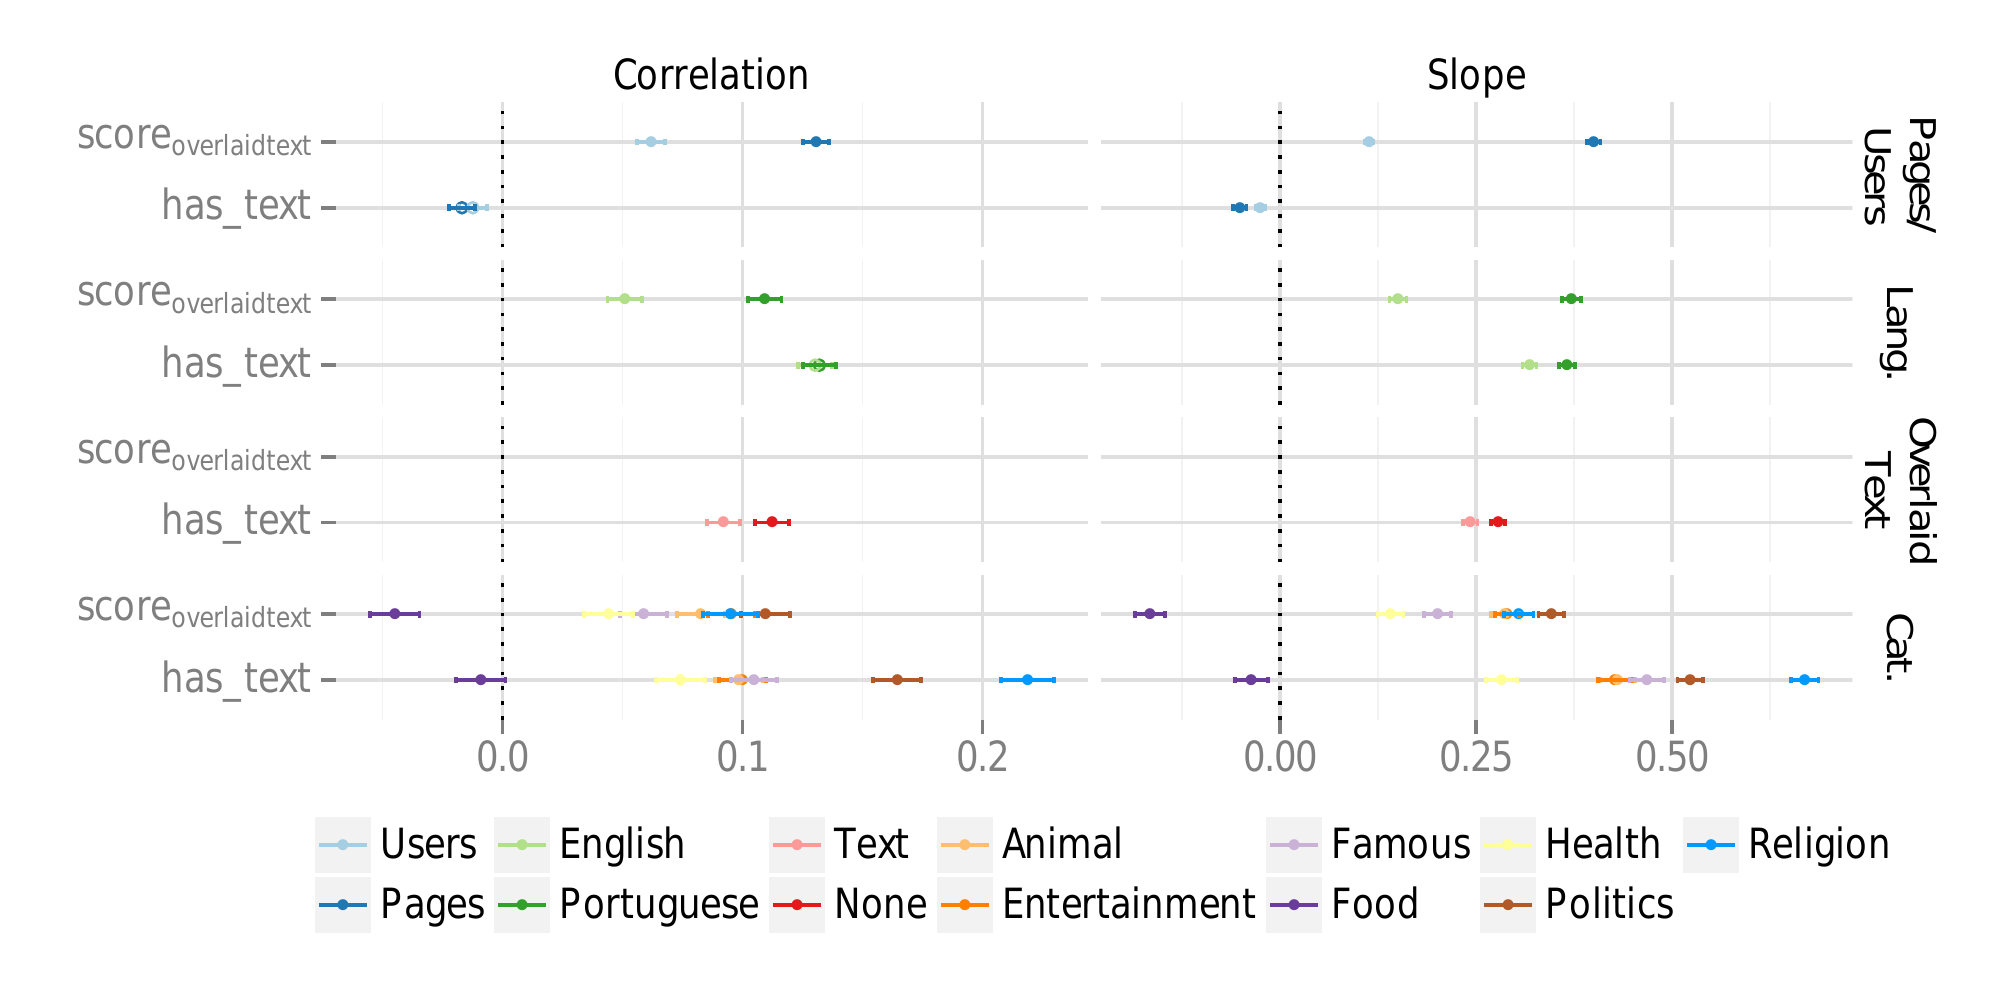}
\caption{Textual features are also beneficial, but only in certain categories.}
\label{fig:cmp_text}
\end{figure}

\begin{figure}
\centering
\includegraphics[width=\linewidth]{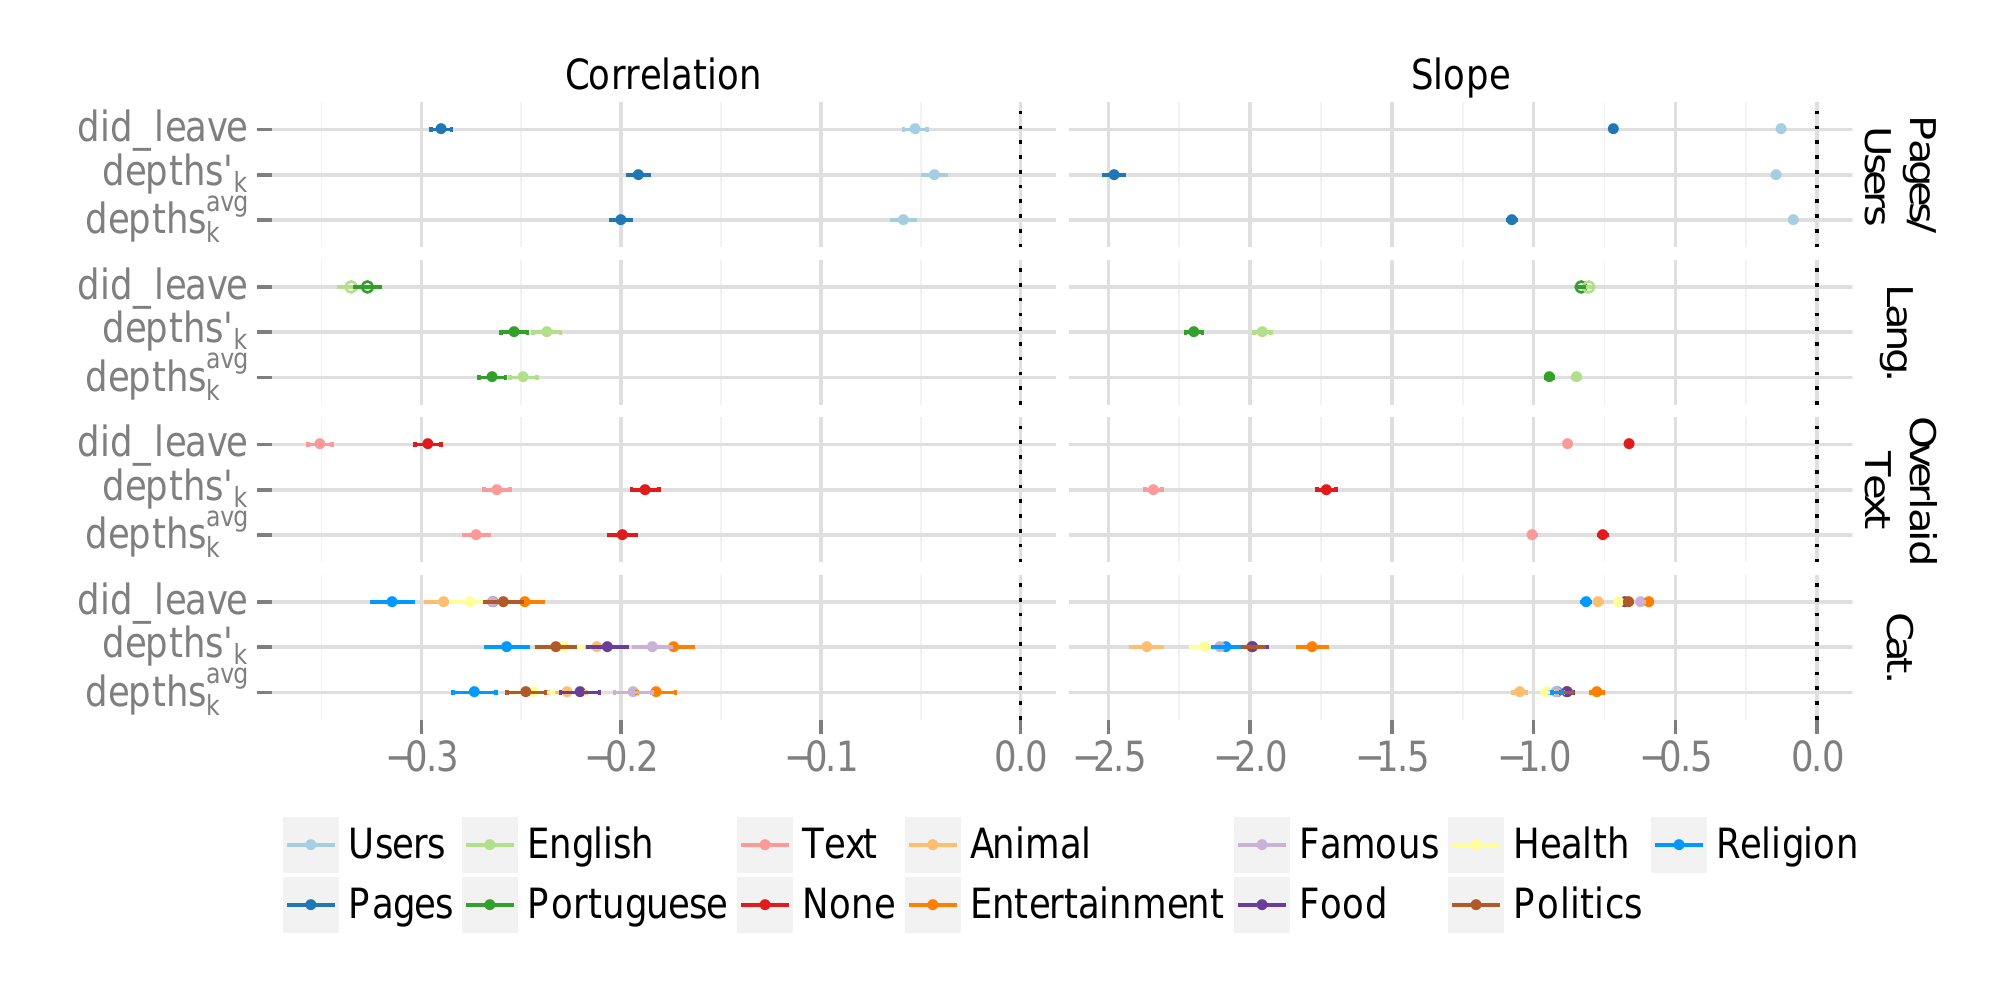}
\caption{Cascade structure also differs among datasets.}
\label{fig:cmp_depth}
\end{figure}

\begin{figure}
\centering
\includegraphics[width=\linewidth]{paper_cmp_text_log}
\caption{Textual features also differ among datasets.}
\label{fig:cmp_depth}
\end{figure}
